# Supplementary material for: Clio: A Hardware-Software Co-Designed Disaggregated Memory System
Source: arXiv:2108.03492 source file (2022-01-20)
Supplement: Supplementary file 1 [file asplos-appendix.tex]

\appendix
\section{Artifact Appendix}

\subsection{Abstract}
This artifact provides the source code of Clio, a hardware-software co-designed disaggregated memory system. The Clio artifact has a C-based host-side library, a C-based ARM SoC management path, and a SpinalHDL-based FPGA data path along with a set of comprehensive FPGA building scripts. The artifact suite also has a set of microbenchmark examples and ported applications.

To run Clio, one needs at least a server equipped with a Mellanox RDMA NIC, a Top-of-Rack switch, and a Xilinx ZCU106 board. Since the FPGA boards are not widely available, we provide a testing bed for the evaluators. The testbed is in our university machine room. To avoid the lengthy FPGA compilation, we pre-setup the testbed with a properly configured host and a configured FPGA board. As an evaluator, you only need to run bash scripts on normal servers.

We selected in total five representative tests to reproduce. These tests showcase Clio's main design points and improvements over existing hardware. We expect reviewers to reproduce at least the same trend and conclusion as presented in our papers. The particular numbers may differ, as we have retired our old 40Gbps VPI switch (which is what we used for the paper submission) and moved to a new 100Gbps Ethernet ToR switch.

\subsection{Artifact Check-List (Meta-information)}
{\small
\begin{itemize}
  \item {\bf Program: }We produce an x86 binary for host, an FPGA bitstream and an ARM binary for SoC. We use YCSB to generate KVS traces.
  \item {\bf Compilation: }We require two GCC instances, one for x86 and another for ARM, both should be higher than version 8.0. We use Scala and Xilinx Vivado to compile FPGA files.
  \item {\bf Run-time environment: } Our host side software require root access, in particular, to access the serial console from FPGA and be able to configure huge page. We have tested our software on Ubuntu 20.04 and CentOS 7.
  \item {\bf Hardware: }The server side requires a Mellanox RDMA NIC, preferably ConnectX-4 and above. Clio's FPGA part can only run on the Xilinx ZCU106 development board.
  \item {\bf Output: }Application run-time latency and throughput.
  \item {\bf Experiments: }The artifact contains a set of scripts and testing cases to reproduce the paper results.
  \item {\bf Publicly available: }\url{https://github.com/WukLab/Clio}
  %\item {\bf Code licenses (if publicly available)?: }
  \item {\bf Archived (DOI): }\url{https://doi.org/10.5281/zenodo.5746392}
\end{itemize}
}

%%%%%%%%%%%%%%%%%%%%%%%%%%%%%%%%%%%%%%%%%%%%%%%%%%%%%%%%%%%%%%%%%%%%%
\subsection{Description}

\subsubsection{How to access}
We archive the source code at \url{https://doi.org/10.5281/zenodo.5746392}.
For the latest version, please access our Github page at \url{https://github.com/WukLab/Clio}.

\subsubsection{Hardware dependencies}
This artifact expects to use the following hardware:
x86 servers equipped with Mellanox RDMA NICs and Xilinx ZCU106 boards.

\subsubsection{Software dependencies}
The following list describes the software dependencies.
{\small
\begin{itemize}
  \item{\bf OS: }Ubuntu 20.04 or CentOS 7.
  \item{\bf Compiler: }gcc-8.0 and above; Scala; Vivado.
  \item{\bf Tool: }PetaLinux.
  \item{\bf Dependent Libraries: }libibverbs.
\end{itemize}
}

%%%%%%%%%%%%%%%%%%%%%%%%%%%%%%%%%%%%%%%%%%%%%%%%%%%%%%%%%%%%%%%%%%%%%
\subsection{Installation}
Users are expected to compile three major parts for a freshly downloaded Clio artifact. The detailed compilation and installation flow is documented at \url{https://github.com/WukLab/Clio/blob/master/Documentation/compile.md}.

%%%%%%%%%%%%%%%%%%%%%%%%%%%%%%%%%%%%%%%%%%%%%%%%%%%%%%%%%%%%%%%%%%%%%
\subsection{Experiment workflow}
To use this artifact, users first need to compile all major components and deploy them. The overall deployment flow is:
1) Use PetaLinux to download the bitstream and a Linux image onto the FPGA board. 2) Download the ARM SoC management binary onto the board. 3) Run test programs on hosts.

%%%%%%%%%%%%%%%%%%%%%%%%%%%%%%%%%%%%%%%%%%%%%%%%%%%%%%%%%%%%%%%%%%%%%
\subsection{Evaluation and expected results}

Clio is a complicated system with many moving parts. To set up Clio from scratch (i.e., from our FPGA source code and a vanilla FPGA board), one would need to deal with low-level FPGA compilation, configuration, and tuning, which is lengthy and error-prone, even to FPGA experts. To make the evaluation process smoother, we decided to pre-setup the whole system including the host side test program and the FPGA boards. As an evaluator, you only need to run bash scripts on normal servers.

Our paper has many results ranging from end-to-end microbenchmark, on-board testing, and end-to-end applications. On-board tests and application evaluation are not easy to setup and require evaluators to play around FPGA directly. Hence, we deciede to only include microbenchmark in the Artifact Evaluation process. These microbenchmark tests cover latency, throughput, and scalability of the Clio system and are representative enough to showcase what our system is capable of and its limitations.

To access testing scripts, please refer to our GitHub documentation at \url{https://github.com/WukLab/Clio/blob/master/Documentation/asplos-ae.md}.

%%%%%%%%%%%%%%%%%%%%%%%%%%%%%%%%%%%%%%%%%%%%%%%%%%%%%%%%%%%%%%%%%%%%%

%\subsection{Note}
%\subsubsection{Port Clio to Other FPGA Boards}

\newpage
